# Supplementary material for: On Expansion and Contraction of DL-Lite Knowledge Bases
Source: arXiv:2001.09365 source file (2020-01-25)
Supplement: Supplementary file 1 [file appendix.tex]

\appendix

%%%% For Section 3.1 %%%%%%%%%%%%%%%%%%%%%%%%%%%%%%%%%%%%%%%%%%%%%%%
\section{Proofs for Section~\ref{sec:mbas}}
\label{sec:append-ModelBasedAproaches}
%%%%%%%%%%%%%%%%%%%%%%%%%%%%%%%%%%%%%%%%%%%%%%%%%%%%%%%%%%%%%%%%%%%%

% \input{proofs/for_section_31/def-for-dalal-op}
% \input{proofs/for_section_31/thm-revision_op_unexpressible}
%
% This is material on topics that are not even mentioned in the core paper

%%%% For Section 3.2 %%%%%%%%%%%%%%%%%%%%%%%%%%%%%%%%%%%%%%%%%%%%%%%
\section{Proofs for Section~\ref{sec:FormulaBasedApproaches}}
\label{sec:append-FormulaBasedAproaches}
%%%%%%%%%%%%%%%%%%%%%%%%%%%%%%%%%%%%%%%%%%%%%%%%%%%%%%%%%%%%%%%%%%%%

% \input{proofs/for_section_32/thm-widtio-coNPcomp} % Full proof is in the paper

%\ftheorem{th:semantics-correctness}
%{
%  The algorithm  $\KU$ runs in polynomial time in input size and 
%  computes evolution according to \BS correctly, i.e.,
%  $\KU(\K,\N)=\upd{\K}{\N}$.
%}
%
%\begin{proof}
%smth
%%
%\qed
%\end{proof}

\ftheorem{th:max-card-np-hard}
{
	For \dlfr TBoxes $\T$, $\T'$ and $\N_T$,
	deciding whether $\T'$ is a maximal by cardinality subset of $\T$ satisfiable
	with $\N_T$ is \nptime-complete.
}

\begin{proof}
smth
\qed
\end{proof}

\ftheorem{th:global-maximum}
{
	For \dlfr KBs $\K$ and $\N$, 
	and ABoxes $\A$
	deciding whether for some TBox $\T$ it holds that 
	$(\T,\A)\in\GMT(\K,\M)$ by set inclusion 
	and by cardinality is
	\nptime-hard, \conptime-hard
	and in $\nptime\cap\conptime$.
}

\begin{proof}
smth
\qed
\end{proof}

%%%% For Section 4.1 %%%%%%%%%%%%%%%%%%%%%%%%%%%%%%%%%%%%%%%%%%%%%%%
\section{Proofs for Section~\ref{sec:ComputingABoxUpdates}}
\label{sec:append-ComputingABoxUpdates}
%%%%%%%%%%%%%%%%%%%%%%%%%%%%%%%%%%%%%%%%%%%%%%%%%%%%%%%%%%%%%%%%%%%%

%!TEX root = /Users/evgenykharlamov/Documents/Bolzano/PhD/2 Writings/Conferences/2010_Mendelzon_Workshop/2010mendelzonworkshop/mainevgeny.tex

%%%%%%%%%%%%%
\flemma{lem:binary-unsatisfiability}
 {
  Let $(\T,\A)$ be a \dllite KB.
  If $(\T,\A)$ is unsatisfiable, 
  then there is a subset $\A_0\incl\A$ with at most two elements, 
  such that $(\T,\A_0)$ is unsatisfiable.
 }

\begin{proof}[Sketch]
	To see this, we consider first TBoxes without functionality assertions.
	Then $\K$ is satisfiable if and only if the Skolemized version of $\K$, say
	$\K'$, is satisfiable.  The set $\K'$ is a set of Horn clauses. It is known
	that, if such a set is unsatisfiable, there is a subset with exactly one
	negative clause that is unsatisfiable.  The only negative clauses in $\K'$ are
	denials that stem from disjointness axioms of the form $A\ISA\lnot B$.
	Suppose that $\K'$ is unsatisfiable and that $\K'_0$ is an unsatisfiable subset
	with at most one negative clause stemming from $B\ISA\lnot C$.  Then, because
	of the form of the assertions in $\T$, there are membership assertions
	$B_0(a)$, $C_0(a)$ in $\K'_0$, for unary concepts $B_0$ and $C_0$ such that
	$\T\models B0\ISA B$ and $\T\models C_0\ISA C$. (Actually, instead of $B_0(a)$
	and $C_0(a)$, we can also have assertions of the form $P_1(a,x)$, $P_2(a,y)$.)

	If we consider also functionality assertions, the claim still holds. In this
	case, the only relevant negative clauses are the ones of the form $a\neq b$,
	for distinct constants $a$ and $b$, which are given implicitly, due to the
	unique name assumption.  They can lead to a contradiction by the interplay with
	functionality and role membership assertions. Again, no more than two role
	membership assertions are needed to give rise to a contradiction.
\qed
\end{proof}
%!TEX root = /Users/evgenykharlamov/Documents/Bolzano/PhD/2 Writings/Conferences/2010_Mendelzon_Workshop/2010mendelzonworkshop/mainevgeny.tex

\ftheorem{thm:bold-semantics-abox-unique}
{
   The result of ABox evolution $\aupd{(\T,\A)}{\N_A}$
 	is uniquely defined.
}

\begin{proof}
	We can construct the unique maximal element $\A_m$ as
	\[
	  \A_m = \{F\in\cl_\T(\A) \mid \{F\} \text{ is $\T$-compatible with } \U \}.
	\]
	To prove that $\A_m$ is $\T$-compatible with $\U$, by
	Lemma~\ref{lem:binary-unsatisfiability}, we only have to show that for each
	$\F\incl\A_m\cup\U$ of at most two elements, $(\T,\F)$ is satisfiable.  If
	$\F=\{F\}$, then either $F\in\cl_\T(\A)$ or $F\in\U$, and since both $(\T,\A)$
	and $(\T,\U)$ are satisfiable, also $(\T,\{F\})$ is satisfiable.  Let's
	consider the case where $\F=\{F_1,F_2\}$.  If $\F\incl\cl_\T(\A)$ or
	$\F\incl\U$, we can argue as before.  Instead, if $F_1\in\cl_\T(\A)$ and
	$F_2\in\U$, then $(\T,\F)$ is satisfiable because by definition of $\A_m$ we
	have that $\{F_1\}$ is $\T$-compatible with $\U$.

	To see that $\A_m$ is also maximal, assume that $A_m\incl\A'\incl\A$ and that
	also $(\T,\A')$ is satisfiable.  Then, for every $F\in\A'$, we have that
	$\{F\}$ is $\T$-compatible with $\U$, hence $F\in\A_m$.  Thus $\A'\incl\A_m$.
\qed
\end{proof}

%!TEX root = /Users/evgenykharlamov/Documents/Bolzano/PhD/2 Writings/Conferences/2010_Mendelzon_Workshop/2010mendelzonworkshop/mainevgeny.tex

%\ftheorem{thm:compute-naive-semantics}
%{  
%  The algorithm  $\AU$ runs in polynomial time in input size and 
%  computes evolution according to \BS correctly, i.e.,
%  $\AU(\K,\N_A)=\upd{\K}{\N_A}$.
%}

\begin{proof}[Sketch]
The fact that \KU returns a maximal non-contradicting set of assertions
follows from the construction of the algorithm.  In Lines~[1]--[9] of \KU, all
atoms that are responsible for unsatisfiability of $(\T,\A\cup\U)$ are detected
and deleted from $\A$ by means of $\weeding$.  The resulting set, say $\S$, is
non-contradicting by construction.  The set is also maximal, because if one
adds to $\S$ any of the assertions of $\cl_\T(\A)$ deleted by $\weeding$, then
this assertion, say $F$, will $\T$-entail either an assertion $B(c)$ such that
$\lnot B(c)$ is $\T$-entailed by $\U$, or $R(a,b)$ such that $R(a,c)$ is
$\T$-entailed by $\U$ and $R$ is functional in $\T$.  Hence, we would get a set
$\S\cup\{F\}$ such that $(\T,\S\cup\{F\})$ is unsatisfiable.
Polynomiality of \KU follows from polynomiality of computing $\cl(\T)$ and
$\cl_\T(\A)$ and of $\weeding$.
\qed
\end{proof}

%%%% For Section 4.2 %%%%%%%%%%%%%%%%%%%%%%%%%%%%%%%%%%%%%%%%%%%%%%%
\section{Proofs for Section~\ref{sec:ComputingCarefulABoxUpdates}}
\label{sec:append-ComputingCarefulABoxUpdates}
%%%%%%%%%%%%%%%%%%%%%%%%%%%%%%%%%%%%%%%%%%%%%%%%%%%%%%%%%%%%%%%%%%%%

%\input{proofs/for_section_42/thm-car_semantics_unique}
%\input{proofs/for_section_42/thm-car_evol_correct}

%%%% For Section 5.1 %%%%%%%%%%%%%%%%%%%%%%%%%%%%%%%%%%%%%%%%%%%%%%%
\section{Proofs for Section~\ref{sec:UpdateAndRevisionPostulates}}
\label{sec:append-UpdateAndRevisionPostulates}
%%%%%%%%%%%%%%%%%%%%%%%%%%%%%%%%%%%%%%%%%%%%%%%%%%%%%%%%%%%%%%%%%%%%

%!TEX root = /Users/evgenykharlamov/Documents/Bolzano/PhD/2 Writings/Conferences/2010_ISWC/2010iswc/evgenymain.tex

\ftheorem{thm:bold-vs-update-revision-postulates}
{
  \BS satisfies postulates \upos{1}-\upos{3} and \rpos{1}-\rpos{3}.
  It also satisfies \upos{4}-\upos{6} and \rpos{4}-\rpos{6} 
  iff a maximal subset $\K_m$ of $\K$, satisfiable with $\N$,
  is unique (up to equivalence),
  where $\K$ is a DL-Lite KB and $\N$ is a new information.
}

%%%%%%%%%%%%%%%%%%%%%%%%%%%%%%%%%%%%%%%%%%%%%%%%%%%%%%%%%%%%%%%%%%
\begin{proof}
First let us prove that $\boldop$ satisfies \upos{1}-\upos{3}.
Since in general $\K_m$ is not unique, we will designate \emph{some $\K_m$} as $\K_m^{(0)}$.

%%%%%%%%%%%%%%%%%%%%%%
\paragraph{\upos{1}:}
By the definition of $\boldop$, 
  $\K \boldop \N = \K_m^{(0)} \cup \N$, and it entails $\N$.

%%%%%%%%%%%%%%%%%%%%%%
\paragraph{\upos{2}:}
Let $\K \models \N$ and $\K$ is satisfiable,
  then it is clear that $\Mod(\K) \cap \Mod(\N) = \Mod(\K)$ and $\K \cup \N$ is satisfiable, 
  so here we have unique $\K_m$ which is equal to $\K$.
Hence, we have:
\begin{align*}
  \Mod(\K \boldop \N) & = &
  \Mod(\K \cup \N) & = &
  \Mod(\K) \cap \Mod(\N) & = &
  \Mod(\K),
\end{align*}
and, consequently, $\boldop$ satisfies \upos{2}.
%
%\dima{General assumption that $\K$ is satisfiable.}

%%%%%%%%%%%%%%%%%%%%%%
\paragraph{\upos{3}:}
By definition of \BS, $\K \boldop \N = \K_m^{(0)} \cup \N$, where $\K_m^{(0)}$ is satisfiable with $\N$,
  whatever $\K_m^{(0)}$ we pick up.
Thus, $\K \boldop \N$ is satisfiable.

\bigskip

Now, suppose that $\K_m$ is unique.
Let us prove that $\boldop$ satisfies \upos{4}-\upos{6}.

%%%%%%%%%%%%%%%%%%%%%%
\paragraph{\upos{4}:}
Let $\K_1 \equiv \K_2$ and $\N_1 \equiv \N_2$
  and $\K_1 \boldop \N_1 = \K_{1m} \cup \N_1$ and $\K_2 \boldop \N_2 = \K_{2m} \cup \N_2$.
To prove that $\K_1 \boldop \N_1 \equiv \K_2 \boldop \N_2$,
  it is enough to show that $\K_{1m} \equiv \K_{2m}$.
Let us show this.

Suppose $\K_{1m} \not\equiv \K_{2m}$, so there exists a DL-Lite KB assertion $\phi$ such that
  $\K_{1m} \models \phi$ and $\K_{2m} \not\models \phi$.
Then, $\K_1 \models \phi$ due to $\K_{1m} \incl \K_1$,
  and $\K_2 \models \phi$ due to $\K_1 \equiv \K_2$.
Since $\K_{2m} \not\models \phi$, it means that $\phi$ was ``dropped'' from $\K_2$ when constructing $\K_{2m}$,
  that is, $\set{\phi} \cup \N_2$ is unsatisfiable.
The latter statement yields that $\set{\phi} \cup \N_1$ is unsatisfiable due to $\N_1 \equiv \N_2$,
  which is impossible since $\phi$ is entailed by $\K_{1m}$ and $\K_{1m} \cup \N_1$ is satisfiable.
Therefore, we have a contradiction and there is no such $\phi$, that is, $\K_{2m} \models \K_{1m}$.
Similarly, one can show that $\K_{1m} \models \K_{2m}$.
Thus, $\K_{1m} \equiv \K_{2m}$.

%%%%%%%%%%%%%%%%%%%%%%
\paragraph{\upos{5}:}
Let $(\K \boldop \N) \cup \K' = \K_m \cup \N \cup \K'$ and $\K \boldop (\N \cup \K') = \K_{m}' \cup \N \cup \K'$,
  where $\K_m$ is the maximal subset of $\K$, satisfiable with $\N$, and
  $\K_m'$ is the maximal subset of $\K$, satisfiable with $\N \cup \K'$.
The latter statement means that $\K_m'$ is satisfiable with $\N$,
  hence, $\K_m' \incl \K_m$ due to the maximality of $\K_m$.
Therefore, $\K_{m}' \cup \N \cup \K' \incl \K_m \cup \N \cup \K'$,
  so $\K_m \cup \N \cup \K' \models \K_{m}' \cup \N \cup \K'$,
  that is,
  $(\K \boldop \N) \cup \K' \models \K \boldop (\N \cup \K')$.

%%%%%%%%%%%%%%%%%%%%%%
\paragraph{\upos{6}:}\
Let $\K \boldop \N_1 = \K_m^1 \cup \N_1$ and $\K \boldop \N_2 = \K_m^2 \cup \N_2$,
  where $\K_m^1$ (resp., $\K_m^2$) is a unique maximal 
  subset of $\K$, satisfiable with $\N_1$ (resp., with $\N_2$).
The condition $\K_m^1 \cup \N_1 \models \N_2$ yields $\K_m^1 \cup \N_2$ is satisfiable.
Hence, $\K_m^1 \incl \K_m^2$ due to maximality of $\K_m^2$.
Similarly, one can check that $\K_m^2 \incl \K_m^1$.
Thus, $\K_m^1 = \K_m^2$.

Now we show that  $\K_m^2 \cup \N_2 \models \K_m^1 \cup \N_1$.
Suppose $\K_m^1 \cup \N_1 \models \phi$ and let $\S$ be a maximal subset of $\K_m^1 \cup \N_1$
  such that $\S \models \phi$.
Then, we can represent $\S$ as an union $\S_1 \cup \S_2$, where $\S_1 \incl \K_m^1$ and $\S_2 \incl \N_1$.
The former inclusion leads to $\S_1 \incl \K_m^2$, since $\K_m^1 = \K_m^2$.
The latter inclusion leads to $\K_m^2 \cup \N_2 \models \S_2$, due to $\K \boldop \N_2 \models \N_1$.
So, $\S_1 \incl \K_m^2$ and $\K_m^2 \cup \N_2 \models \S_2$ means that
  $\K_m^2 \cup \N_2 \models \S$, that is, $\K_m^2 \cup \N_2 \models \phi$.
Hence, $\K_m^2 \cup \N_2 \models \K_m^1 \cup \N_1$.
Similarly, one can show that $\K_m^1 \cup \N_1 \models \K_m^2 \cup \N_2$.
Thus, $\K \boldop \N_1 \equiv \K \boldop \N_2$.

\bigskip

Before showing that \upos{4}-\upos{6} do not hold if $\K_m$ is not unique,
  we should define the meaning of an expression $\K \boldop \N \equiv \S$ for some $\S$.
The point is that $\K \boldop \N$ is \emph{not a deterministic set} 
  and the result of update of the same KB with the same new information 
  may differ when we do it two times.
So, we say that $\K \boldop \N \equiv \S$ if and only if $\K_m^{(0)} \cup \N \equiv \S$
  for \emph{every} maximal subset $\K_m^{(0)}$.
  
\bigskip

Now, we consider \upos{4}-\upos{6}.

For \upos{4}, we can consider the case when $\K_1 = \K_2 = \K$ and $\N_1 = \N_2 = \N$.
Then, if we have two maximal subsets $\K_m^{(1)}$ and $\K_m^{(2)}$,
  then it is clear that $\K_1 \boldop \N_1 \not\equiv \K_2 \boldop \N_2$,
  since $\K_m^{(1)} \not\equiv \K_m^{(2)}$.
  
Similarly for \upos{5}, it may be a case that $\K_m' \not\incl \K_m$
  (notation here follows the notation of the corresponding paragraph),
  since $\K_m'$ may be a subset of another $\K_m^{(1)}$, which is maximal for $\N$
  and different from $\K_m$.
Thus, $\boldop$ does not satisfy \upos{5} in general.

Analogously to the previous case, $\boldop$ does not satisfy \upos{6}.
%

%%%%%%%%%%%%%%%%%%%%%%%%%%%%%%%%%%%%%%%%%%%%%%%%%%%%%%%%%%%%%%%%%%

First let us prove that $\boldop$ satisfies \rpos{1}-\rpos{3}.
Since in general $\K_m$ is not unique, we will designate \emph{some $\K_m$} as $\K_m^{(0)}$.

%%%%%%%%%%%%%%%%%%%%%%
\paragraph{\rpos{1}, \rpos{3}:} 
The proof of satisfiability $\boldop$ to these two postulates
  mimic the corresponding proof for \upos{1}, \upos{3} in Theorem~\ref{thm:bold-upos}.

%%%%%%%%%%%%%%%%%%%%%%
\paragraph{\rpos{2}:}
This one follows from the definition of $\boldop$ and the fact that 
  if $\K \cup \N$ is satisfiable, then $\K_m = \K$.

\bigskip

Now, suppose that $\K_m$ is unique.
Let us prove that $\boldop$ satisfies \upos{4}-\upos{6}.

%%%%%%%%%%%%%%%%%%%%%%
\paragraph{\rpos{4}, \rpos{5}:}
The proof of satisfiability $\boldop$ to these two postulates
  mimic the corresponding proof for \upos{4}, \upos{5} in Theorem~\ref{thm:bold-upos}.

%%%%%%%%%%%%%%%%%%%%%%
\paragraph{\rpos{6}:}
Let $(\K \boldop \N) \cup \K' = \K_m \cup \N \cup \K'$ and $\K \boldop (\N \cup \K') = \K_{m}' \cup \N \cup \K'$,
  where $\K_m$ is the maximal subset of $\K$, satisfiable with $\N$, and
  $\K_m'$ is the maximal subset of $\K$, satisfiable with $\N \cup \K'$.
Let $(\K \boldop \N) \cup \K'$ be satisfiable, that is, $\K_m$ is satisfiable with $\N \cup \K'$.
Hence, $\K_m \incl \K_m'$ due to maximality of $\K_m'$, therefore,
  $\K_m \cup \N \cup \K' \incl \K_{m}' \cup \N \cup \K'$, that is,
  $\K_m' \cup \N \cup \K' \models \K_m \cup \N \cup \K'$, and
  $\boldop$ satisfies \rpos{6}.
  
\bigskip

If $\K_m$ is not unique, then $\boldop$ does not satisfy \rpos{4}-\rpos{6}.
This can be shown similarly as it is shown in Theorem~\ref{thm:bold-upos}
  that $\boldop$ does not satisfy \upos{4}-\upos{6}.
\qed

\end{proof}

\begin{lemma}
\label{lemma:abox-closure-and-tbox-equivalency}
Let $\K_1 = \lrbr{\T_1, \A_1}$ and $\K_2 = \lrbr{\T_2, \A_2}$ be two DL-Lite KBs
  such that $\K_1 \equiv \K_2$.
Then 

\begin{compactenum}[(a)]
	\item $\T_1 \equiv \T_2$, and 
	\item $\cl_{\T_1}(\A_1) = \cl_{\T_2}(\A_2)$.
\end{compactenum}
\end{lemma}

\begin{proof}
Let us first prove that $\T_1 \equiv \T_2$.
Suppose it is not the case,
  so there is a DL-Lite assertion $f$ such that $\T_1 \models f$ and $\T_2 \not\models f$
  (symmetrically, $\T_2 \models f$ and $\T_1 \not\models f$).
There are three options:
\begin{compactenum}
	\item\label{concincl}
	       $f = B \ISA C$,
	\item\label{roleincl}
	       $f = Q \ISA R$, and
	\item\label{functass}
	       $f = (\funct\ R$).
\end{compactenum}
Any of these cases leads to contradiction.
To show this, we take a model $\J$ of $\K_2$ and construct from it a model $\J'$
  such that $\J'$ is a model of $\K_2$ and not a model of $\K_1$,
  which contradicts to the equivalence of $\K_1$ and $\K_2$.

In Case~\ref{concincl}, we construct $\J'$ 
  setting $a_{B \ISA C} \in B^{\J'}$ and $a_{B \ISA C} \notin C^{\J'}$,
  where $a_{B \ISA C}$ is a fresh constant, that did not appear in the $\J$ before.
By construction, $\J'$ is a model of $\T_2$ and not a model of $\T_1$.
Since $a_{B \ISA C}$ did not appear in $\J$, so $\J'$ does not contradict to $\A_2$.
Thus, we have that $\J' \in \Mod(\T_2) \cap \Mod(A_2) = \Mod(K_2)$,
  and $\J' \notin \Mod(K_1)$, since $\J' \notin \Mod(\T_1)$.
Contradiction with equality of $\K_1$ and $\K_2$.

In Case~\ref{roleincl}, we do the similar thing:
  we construct a model $\J'$, 
  setting $(a_{Q \ISA R}, b_{Q \ISA R}) \in Q^{\J'}$
  and $(a_{Q \ISA R}, b_{Q \ISA R}) \notin R^{\J'}$,
  where $a_{Q \ISA R}$ and $b_{Q \ISA R}$ are fresh constants.
It is easy to see that $\J' \in \Mod(\K_2) \setminus \Mod(\K_1)$,
  which contradicts to the equivalence of $\K_1$ and $\K_2$.
  
Finally, in Case~\ref{functass}, we construct $\J'$, 
  setting $(a_R, b_R) \in R^{\J'}$ and $(a_R, c_R) \in R^{\J'}$,
  where $a_R$, $b_R$, and $c_R$ are fresh constants.
It is easy to see that $\J' \in \Mod(\K_2) \setminus \Mod(\K_1)$,
  which contradicts to the equivalence of $\K_1$ and $\K_2$.
  
Thus, $\T_1 \equiv \T_2$.

Now we prove that $\cl_{\T_1}(\A_1) = \cl_{\T_2}(\A_2)$.
By the definition of  closure of an ABox,
  $\cl_{\T_i}(\A_i)$ is a set of all memberdhip assertions $f$ over the constants in $\adom(\A_i)$
  such that $\lrbr{\T_i, \A_i} \models f$,
  where $i = 1, 2$.

Suppose $f \in \cl_{\T_1}(\A_1)$, that is, $\lrbr{\T_1, \A_1} \models f$.
This means that $\K_1 \models f$ and due to the equivalence of  $\K_1$ and $\K_2$,
  it holds that $\K_2 \models f$, that is, $\lrbr{\T_2, \A_2} \models f$,
  that is, $f \in \cl_{\T_2}(\A_2)$.
  
Similarly, one can check that for every $f$ in $\cl_{\T_2}(\A_2)$,
  it holds that $f \in \cl_{\T_1}(\A_1)$.
Thus, $\cl_{\T_1}(\A_1) = \cl_{\T_2}(\A_2)$.
\qed
\end{proof}

%%%%%%%%%%%%%%%%%%%%%%%%%%%%%%%%%%%%%%%%%%%%%%%%%%%%%%%%%%%%%%%%%
%%%%%%%%%%%%%%%%%%%%%%%%%%%%%%%%%%%%%%%%%%%%%%%%%%%%%%%%%%%%%%%%%

%%%% For Section 5.2 %%%%%%%%%%%%%%%%%%%%%%%%%%%%%%%%%%%%%%%%%%%%%%%
\section{Proofs for Section~\ref{sec:comparison-semantics}}
\label{sec:append-UpdateAndRevisionPostulates}
%%%%%%%%%%%%%%%%%%%%%%%%%%%%%%%%%%%%%%%%%%%%%%%%%%%%%%%%%%%%%%%%%%%%

\fproposition{prop:entailment-preservation}
{
Let $(\T,\A)$ be a \dlfr KB and 
  $\N_A$ be a set of ABox assertions satisfiable with $\T$.  
  \begin{compactenum}
  \item If $\N_A \tmodels \varphi$,
        then $\A'_b \tmodels \varphi$ and $\A'_c \tmodels \varphi$, 
		for any \FOL formula $\varphi$.  
  \item If $\N_A\not\tmodels \varphi$ and $\N_A \not\tmodels \lnot\varphi$, then
  		\begin{compactenum}[(i)]
  			\item if $\A \tmodels \varphi$, then $\A'_b \tmodels \varphi$, 
					when $\varphi$ is an ABox assertion, and
  			\item if $\A \not \tmodels \varphi$, 
				  then $\A'_c \not \tmodels \varphi$, when
    			  $\varphi$ is an ABox assertion or role-constraining.
  		\end{compactenum}
  \end{compactenum}
}

\endinput

%%% Local Variables:
%%% mode: latex
%%% TeX-master: "main"
%%% End:
